# Supplementary material for: Transparency versus Anderson localization in one-dimensional disordered stealthy hyperuniform layered media
Source: arXiv:2507.22377 ancillary file (2025-07-30)
Supplement: Supplementary file 1 [file supplementary.pdf]

# Supplementary Materials for Transparency versus Anderson localization in one-dimensional disordered stealthy hyperuniform layered media

Michael A. Klatt, Paul J. Steinhardt, Salvatore Torquato

July 26, 2025

## $\tau$ -order metric

The  $\tau$ -order metric has been defined to quantify the degree of order across length scales at the two-point level [1]. The  $\tau$ -order metric diverges for the perturbed lattice because of the Bragg peaks, but it can still be used to compare different degrees of order by considering  $\tau(L)$  as a function of system size  $L$  [2, 3, 4]. For a one-dimensional system, the  $\tau$ -order metric is given by:

$$\tau(L) := 2 \int_0^L [g_2(x) - 1]^2 dx, \quad (1)$$

where  $g_2(x)$  is the pair-correlation function. The  $\tau$ -order metric is zero for the ideal gas (i.e., the Poisson point process [5]). It quantifies correlated disorder and picks up both positive and negative correlations at all scales. Hence, it sensitively detects deviations (at the two-point level) from a purely random system.

Table 1 in the main text provides the exact values for the lattice and perturbed lattice; see also [4]. For the other systems, we estimate  $g_2(x)$  from 100 samples for each model using a bin size of 0.1 for  $x > 0.1$  and 0.001 for  $0 < x < 0.1$ . We then, numerically evaluate the integral of (1) above using the composite trapezoidal rule.

## Spectral density

The spectral density  $\tilde{\chi}(k)$  of a two-phase material is the Fourier transform of the autocovariance  $\chi(r)$  [6]. In our setting with non-overlapping equally-sized slabs,  $\tilde{\chi}(k)$  is closely related to the structure factor  $S(k)$  of the original point pattern [7]:

$$\tilde{\chi}(k) = \rho m^2(k) S(k), \quad (2)$$

where  $m(k) = 2 \sin(k\phi/2)/k$  is the Fourier transform of a single slab.

## Issues in interpreting figures of transmission versus frequency

Figure 2 in our paper shows the numerically computed transmission  $T$  as a function of frequency  $\omega$  for various types of layered media. In particular, the upper panel compares the transmission for layers arranged in a perfect (periodic) 1D lattice to transmission computed for disordered stealthy hyperuniform arrangements with different values of  $\chi$ . In each case, the frequency range is limited to  $0 < \omega < \omega_T$ , the range of interest for our study. The calculations are for single samples consisting of 10,000 layers for each type model.

The naive expectation for media with no localization between zero and  $\omega_T$  would be that  $T = 1$  precisely up to  $\omega_T$ . However, for all four cases in Figure 2, including the perfect (periodic) lattice for which it is rigorously known that there is no localization, the plot does not meet this expectation. Instead, what occurs in all four cases but is most visible for the lattice is an apparent shaded region between  $T = 1$  and some curve with  $T < 1$ . This is the ripple effect due to the finite boundary conditions [8]. This effect is also illustrated in the top left panel of Fig. 1. The magnified region shows that the shaded region actually consists of very closely up and down oscillations in  $T$  that are too closely spaced to be resolved in the image in which  $T$  reaches  $T = 1$  in each oscillation. The fact that the disordered stealthy hyperuniform samples appear to have the same behavior is consistent with our claim that there are no apparent signs of localization over the length scales that can be probed numerically.

As represented in the top right and lower left panels of Fig. 1, the ripple effect can cause two other misleading effects if one is not aware of them. The first occurs if one averages over many samples. Because the rippling oscillations are generally slightly different in phase for each sample, the averaged  $T$  curves away from  $T = 1$  as illustrated in the top right panel, giving the false impression of localization. The second effect, illustrated on the bottom left, occurs if there is insufficiently fine sampling of frequencies. Regular rapid rippling oscillations can appear in some cases like wildly variation transmission.

As the frequency of ripple oscillations increases with increasing system size, the first two misleading effects tend to get stronger for larger systems when one might have expected that larger systems would give more precise results. Moreover, they are enhanced as the dielectric contrast gets stronger. For a clear demonstration of these effects, we have used in Fig. 1 a dielectric contrast  $\varepsilon_2/\varepsilon_1 = 16$  and a volume fraction  $\phi = 20\%$  for 10,000 high-dielectric slabs.

A third kind of misleading effect occurs if the incident medium and substrate have dielectric constants different from the low dielectric constant medium separating the slabs with high dielectric constant. In that case, the initial and final reflections can reduce the maximum possible transmission, as illustrated on the bottom right of Fig. 1. If the incident medium and substrate have dielectric constants that are different from each other, then the upper boundary of  $T$  can curve in various ways as well as be suppressed.

Hence, for the reasons summarized in Fig. 1, transmission plots can be difficult to interpret even in cases where there is no localization. Moreover, we find that, because ripple effects are more screened in Lyapunov exponent analyses, computing Lyapunov exponents is more useful for localization analysis.

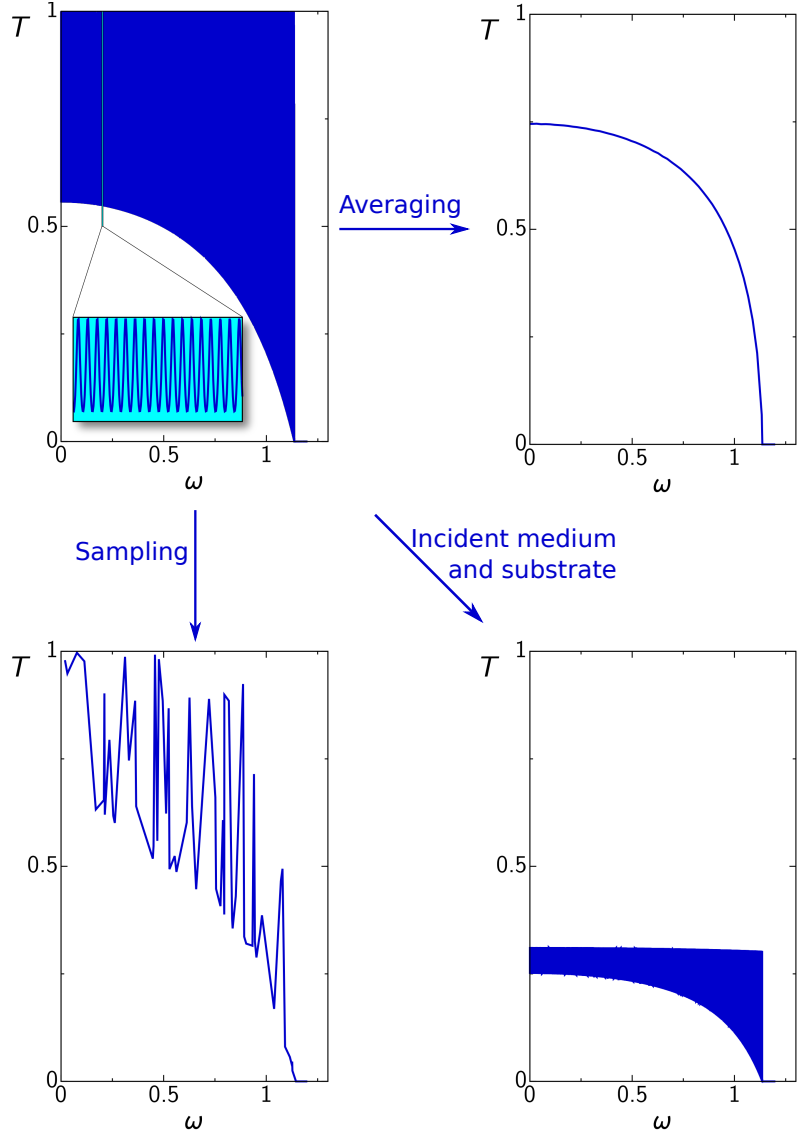

Figure 1: Four issues to contend with in a transmission analysis of localization: all four plots show the transmission coefficient  $T$  as a function of frequency  $\omega$  for 10,000 layers of the integer lattice decorated with high-dielectric slabs with  $\varepsilon_2 = 9$ ,  $\varepsilon_1$  and  $\phi = 50\%$  (chosen to visually enhance the effects). The perfect transparency, however, is obscured by the ripple effect, as shown in the **top left** figure and inset, which turns simple  $T = 1$  behavior into what appears as the blue shaded region bounded above by  $T = 1$  and by a curve below. When magnified the shade region is seen to consist of high frequency “ripple” oscillations with maxima at  $T = 1$ , which is the best that can be obtained even for a perfect lattice with no localization. Because the ripple effect for larger systems causes higher-frequency oscillations, perfect transparency can be obscured due to interference effects if one averages over different samples, as illustrated in (**top right**). As shown on the (**bottom left**),  $T$  appears to undergo wild oscillations if one uses a sampling with a sampling in  $\omega$  that is too low. (Here the sampling has been done with random values of  $\omega$ .) Yet a third issue, arises if the dielectric constant of the incident medium and substrate do not match the  $\varepsilon_1$ , the dielectric constant of the medium separating the slabs. In the example shown in (**bottom right**), the dielectric constant of the incident medium and substrate have been chosen to equal to  $\varepsilon_2$ . The result is an apparent reduction in transmission  $T$  even though the slab medium itself is perfectly transparent.

## References

- [1] S. Torquato, G. Zhang, and F. H. Stillinger. Ensemble Theory for Stealthy Hyperuniform Disordered Ground States. *Phys. Rev. X*, 5:021020, 2015.
- [2] S. Atkinson, F. H. Stillinger, and S. Torquato. Static structural signatures of nearly jammed disordered and ordered hard-sphere packings: Direct correlation function. *Phys. Rev. E*, 94:032902, 2016.
- [3] S. Torquato, G. Zhang, and M. D. Courcy-Ireland. Hidden multiscale order in the primes. *J. Phys. A: Math. Theor.*, 52:135002, 2019.
- [4] M. A. Klatt, J. Kim, and S. Torquato. Cloaking the underlying long-range order of randomly perturbed lattices. *Phys. Rev. E*, 101:032118, 2020.
- [5] G. Last and M. Penrose. *Lectures on the Poisson Process*. Institute of Mathematical Statistics Textbooks. Cambridge University Press, Cambridge, 2017.
- [6] S. Torquato. *Random Heterogeneous Materials*, volume 16 of *Interdisciplinary Applied Mathematics*. Springer, New York, second edition, 2002.
- [7] S. Torquato. Hyperuniform states of matter. *Phys. Rep.*, 745:1–95, 2018.
- [8] H. A. Macleod. *Thin-Film Optical Filters*. CRC Press, Boca Raton; London; New York, fourth edition, 2010.
